# Supplementary material for: Batch Normalization Explained
Source: arXiv:2209.14778 source file (2022-09-29)
Supplement: Supplementary file 1 [file si.tex]

\documentclass[9pt,twoside,lineno]{pnas-new}
% Use the lineno option to display guide line numbers if required.
\input{preamble}
\usepackage{multirow}
\usepackage{xr}
\makeatletter
\newcommand*{\addFileDependency}[1]{% argument=file name and extension
  \typeout{(#1)}
  \@addtofilelist{#1}
  \IfFileExists{#1}{}{\typeout{No file #1.}}
}
\makeatother

\newcommand*{\myexternaldocument}[1]{%
    \externaldocument{#1}%
    \addFileDependency{#1.tex}%
    \addFileDependency{#1.aux}%
}

\myexternaldocument{main}
\templatetype{SI/pnassupportinginfo}
\title{Batch-Normalization, Explained}
\author{Randall~Balestriero and Richard~G.~Baraniuk}
\correspondingauthor{Randall Balestriero.\\E-mail: randallbalestriero@gmail.com}

\begin{document}

%% Comment out or remove this line before generating final copy for submission; this will also remove the warning re: "Consecutive odd pages found".

\maketitle

%% Adds the main heading for the SI text. Comment out this line if you do not have any supporting information text.
\SItext

\input{SI/si_content}

%PROOF FOR VARIAVE OF VARIANCE
%\url{https://math.stackexchange.com/questions/72975/variance-of-sample-variance}

\bibliography{pnas-sample}

\end{document}
